# Supplementary material for: Two-stage Stochastic Matching and Pricing with Applications to Ride Hailing
Source: arXiv:2210.11648 source file (2022-10-21)
Supplement: Supplementary file 1 [file appendix-optonline-unweighted.tex]

Before the proof of \Cref{lem:online final} for the unweighted, we first introduce the following technical lemma 
for structural decomposition.
\begin{lemma}
\label{lem:msc closed form}
In the structural decomposition 
(\Cref{lemma:structure}),
$\mspairci = 
\frac{|\Driveri| - |\Rideri|}{\sum_{j\in\Driveri}\frac{1}{\weight_j}}$.
\end{lemma}
\begin{proof}[\emph{Proof.}]
The uniformity and saturation properties 
in \Cref{lemma:structure}
give a unique closed-form solution $\frac{|\Driveri| - |\Rideri|}{\sum_{j\in\Driveri}\frac{1}{\weight_j}}$ for $\mspairci$.
\end{proof}
\input{tex/stochastic_proof_unweighted.tex}

% Before the proof of \Cref{lem:online final},
% we first show \Cref{thm:opt-online-comp-ratio}
% from \Cref{lem:online final}.
\begin{proof}{\emph{Proof of \Cref{thm:opt-online-comp-ratio}}.}
We evaluate the 
program~\ref{eq:online final} in both 
unweighted and weighted settings. In the former, we further restrict to $\weightp = \weightdp = 1$
in program~\ref{eq:online final}. Therefore, it becomes
\begin{align*}
    \min_{
    \msfirst,\mssecond\in[0, 1]:
    \msfirst +\mssecond \leq 1
    }
    1-
    \frac{
    \combprob\,\msfirst\,\mssecond
    +
    \frac{1}{e}(1-\combprob)\mssecond
    }{\msfirst+\mssecond}~,
\end{align*}
% \AS{fix spacing}
with the optimal value $\onlineUnweightedRatioText$
at $\msfirst =
\tfrac{\combprob-\frac{1}{e}(1-\combprob)}
{2\combprob},
\mssecond = 
\tfrac{\combprob+\frac{1}{e}(1-\combprob)}{2\combprob}$
for $\combprob=\tfrac{1}{(e-1)}$. In the weighted setting, we numerically solve
the program for
cases $\msfirst + \mssecond = 1$
and $\msfirst + \mssecond < 1$.
The optimum value is close to $\onlineWeightedRatio$.\hfill\Halmos
% The first order conditions (FOC) of variable $\mixap$
% and $\weight$ are 
% \begin{align*}
%     \frac{1}{e}(\mixap^2 - e\combprob\mixap + 
%     (e-1)\combprob\mixap^2)\weight^2
%     &+
%     \frac{2}{e}(1-\combprob)\mixap(1-\mixap)\weight\\
%     +
%     \combprob\mixap(1&-\mixap)
%     +
%     \frac{1}{e}(1-\combprob)(1-\mixap)^2 
%     &= 0 \qquad (\text{FOC respect to }\weight)\\
%     (1-\combprob)(\weight-1)^2\mixap^2
%     +
%     2(1-\combprob)(\weight - 1)\mixap
%     &+
%     2e\combprob\weight\mixap
%     -e\combprob\weight
%     +
%     1-\combprob
%     &= 0
%     \qquad (\text{FOC respect to }\mixap)
% \end{align*}
% With $\combprob=0.7$, program \eqref{eq:online final}
% attains its minimum approximately $\onlineWeightedRatio$
% at $\weight\approx 1.36386$ and 
% $\mixap\approx 0.423036$.
\end{proof}
